# Supplementary material for: MRI Reconstruction with Regularized 3D Diffusion Model (R3DM)
Source: arXiv:2412.18723 source file (2024-12-25)
Supplement: Supplementary file 1 [file supplement.tex]

\appendix
\section{Supplementary Materials}\label{sec:supplement}
In this section, we present the supplementary material used to support the main paper. We begin by providing the summary of the analysis of the Diffusion Proximal Projection Method, as well as the strategy to choose step size $\lambda$. Additionally, we discuss supporting materials, including the Fourier slice method, as well as the proximal method and regularization. Here, we adhere to the notation using a one-dimensional vector to align with results in the literature and facilitate the derivation of the analysis of the proposed method.
\subsection{Approximation bound of the Proposed Method} \label{sec:ConvAnalysis}
In this section, we will first discuss the challenge of using the Diffusion Model for reconstructing MR images. Then, we will demonstrate that the existing method is inadequate for 3D data due to its loose bound at high dimensionality of $d=SN^2$. Finally, we will show that our proposed method has a better approximation bound for 3D reconstruction.
\paragraph{\underline{MRI Reconstruction with Diffusion Model}}
% The algorithm proposed in this article contains two processes, namely the \ac{DDPM} sampling and optimization problem in \eqref{eq:opt}. 
In MRI reconstruction, we have a noisy measurement model with Gaussian noise $\mbf n \in \R^d$ as follows
$$
\mbf{y} = \mcl{A}\left(\mbf{x}\right) + \mbf n
$$
The goal of the proposed method is to incorporate under-sampled measurement data $\mbf{y}$, i.e., k-space, to improve the reconstruction image of interest $\mbf x$, i.e., 3D MR images, with diffusion model's sampling process, i.e., reverse {SDE}. Hence, the reverse process in \eqref{eq:reverse_SDE} can be written as
\begin{equation} 
    \mrm{d}\mbf{x} = \left( \mcll{f}\left(\mbf{x}, t \right) \mrm{d}t - \mcll{g}^2\left( t \right) \left(  \nabla_{\mbf x} \log p \left(\mbf{y}|\mbf{x}_t \right) \right) + \nabla_{\mbf x} \log p\left(\mbf{x}_t \right) \right) + \mcll{g}\left( t \right) \mrm{d}\mbf{w}.
\end{equation}
%  and  estimated data $\mbf{x}_t$ at each iteration with \ac{DDPM} sampling, i.e., reverse of SDE, we need to show whether for each reverse time index, we can approximate the true solution. In the sampling process, instead of using the score function $\nabla_{\mbf{x}_0}\log p(\mbf{x}_0)$, the conditional probability density function is incorporated to the sampling process
%$$
%\nabla_{\mbf{x}_0}\log p(\mbf{x}_0|\mbf{y}) = %\nabla_{\mbf{x}_0}\log p(\mbf{x}_0) + %\nabla_{\mbf{x}_0}\log p(\mbf{y}|\mbf{x}_0).%
%$$
Here, $\nabla_{\mbf{x}}\log p(\mbf{x}_t)$ is estimated by using a neural network model $\mcll{s}_{\bs \theta^*}\left(\mbf{x}_t \right)$ for each time index $t$. The challenge is now to find a good approximation strategy to estimate $p\left(\mbf{y}|\mbf{x}_t \right)$. %and $\nabla_{\mbf{x}_0}\log p(\mbf{y}|\mbf{x}_0)$ is approximated by an optimization scheme derived from  $\nabla_{\mbf{x}_t}\log p(\mbf{y}|\mbf{x}_t)$ for each time index $t$. 

\paragraph{\underline{Diffusion Posterior Sampling}} The authors in \cite[Proposition 1]{chung2023diffusion} proposed a method by using DDPM sampling and show that DDPM sampling is a good approximation to estimate  $p\left(\mbf{y}|\mbf{x}_t\right)$. We first restate the result of the DDPM sampling in the following proposition. 
\begin{proposition}{[Proposition 1 in \cite{chung2023diffusion}]}\label{prop:prop1}
For \ac{DDPM} sampling, the conditional probability $p\left(\mbf{x}_0 | \mbf{x}_t\right)$ has unique posterior mean
$$
\mbf{\hat{x}}_0 := \E\left[\mbf{x}_0 | \mbf{x}_t\right] = \frac{1}{\sqrt{\bar \alpha_t}} \left( \mbf{x}_t + \left(1 - \bar{\alpha_t}\right) \nabla_{\mbf{x}_t} \log p\left(\mbf{x}_t \right)\right),
$$
where $\bar{\alpha}_t = \prod_{j=1}^t (1 - \beta_j)$.
\end{proposition}
Proposition \ref{prop:prop1} shows that we can estimate the expected value of reverse \ac{SDE} with \ac{DDPM} sampling.  Hence, taking the result from Proposition \ref{prop:prop1},  $\mbf{\hat{x}}_0 := \E\left[\mbf{x}_0 | \mbf{x}_t\right]$, the authors show $p\left(\mbf{y}|\mbf{x}_t \right) \approx p\left(\mbf{y}|\mbf{\hat{x}}_0 \right)$. The proof strategy is given by rewriting the data fidelity as follows \cite[eq.7]{chung2023diffusion}:
\begin{equation}
\label{eq:cond_exp}
    \begin{aligned}
    p\left(\mbf{y} | \mbf{x}_t\right) &= \int p\left(\mbf{y} | \mbf{x}_0\right) p\left(\mbf{x}_0 | \mbf{x}_t\right) \mathrm{d}\mbf{x}_0 = \E\left[p\left(\mbf{y} | \mbf{x}_0\right)\right].
    \end{aligned}
\end{equation} 
Hence, combining Proposition \ref{prop:prop1} and \eqref{eq:cond_exp}, we have to quantify the approximation of  $\card{p\left(\mbf{y} | \mbf{x}_t\right) - p\left(\mbf{y} | \mbf{\hat x}_0\right)}$. In fact, this quantification is given in Theorem 1 \cite{chung2023diffusion}.
\begin{theorem}{[Theorem 1 in \cite{chung2023diffusion}]}\label{thm:theorem1}
For given measurement model $\mbf{y} = \mcl{A}\left(\mbf{x}_0\right) + \mbf{n}$ where $\mbf{n} \sim \mcl{N}\left(0, \sigma^2\mbf{I}\right)$ and $\mbf{\hat{x}}_0 := \E\left[\mbf{x}_0 | \mbf{x}_t\right]$ from Proposition \ref{prop:prop1},  we have
\begin{equation}
\card{ \E\left[p\left(\mbf{y} | \mbf{x}_0\right)\right]- p\left(\mbf{y} |\textcolor{blue}{\mbf{\hat x}_0}\right)} \leq \textcolor{blue}{\frac{d}{\sqrt{2\pi \sigma^2}} e^{-1/2\sigma^2} }\underset{\mbf{x}}{\text{max}}\norm{\nabla_{\mbf{x}} \mcl{A}\left(\mbf{x}\right)}_2 \textcolor{blue}{m_1},
\end{equation}
where $\textcolor{blue}{m_1} := \E \left[\norm{\mbf{x}_0 - \mbf{\hat x}_0}_2  \right] = \int \norm{\mbf{x}_0 - \mbf{\hat x}_0}_2 p(\mbf{x}_0| \mbf{x}_t) \mathrm{d}\mbf{x}_0$ and $\textcolor{black}{d} $ is total dimension of $\mbf{x}_0$.
\end{theorem}

Intuitively, Theorem \ref{thm:theorem1} measures the error approximation of conditional distribution $ p(\mbf y|\mbf{x}_t) $ with $ p\left(\mbf{y} | \mbf{\hat x}_0\right)$ given the result from the reverse \ac{SDE} in terms of \ac{DDPM} sampling  method, i.e., $\mbf{\hat{x}}_0 := \E\left[\mbf{x}_0 | \mbf{x}_t\right]$. The quantification of error approximation is given by the upper bound $\underset{\mbf{x}}{\text{max}}\norm{\nabla_{\mbf{x}} \mcl{A}\left(\mbf{x}\right)}_2$ and   $m_1 := \E \left[\norm{\mbf{x}_0 - \mbf{\hat x}_0}_2  \right]$, respectively. The first parameter is the maximum norm of the gradient forward operator $\mcl{A}$ that uniquely represents the measurement data, i.e., $\mbf{y} = \mcl{A}\left(\mbf{x} \right) + \mbf{n}$, for all possible input $\mbf{x}$. The second parameter represents the expected value or mean of differences between the posterior mean in Proposition \ref{prop:prop1} and the original data.  The proof strategy utilizes the property of the Jensen gap and the conditional probability density function in terms of Gaussian. The latter holds because the measurement model is incorporated with additive Gaussian noise  $\mbf{n} \sim \mcl{N}\left(0, \sigma^2\mbf{I}\right)$. However, the approximation bound highly depends on the dimension of data $\mbf{x}_0$ which is given in the factor $d$. This could highly affect the approximation if the data dimension is very large, especially for volumetric data where we have a total dimension, for instance, $d = SN^2$.
 %The upper bound depends on the parameters $\underset{\mbf{X}}{\text{max}}\norm{\nabla_{\mbf{X}} \mcl{A}\left(\mbf{X}\right)}$ and  $\E \left[\norm{\mbf{X}_0 - \mbf{\hat X}_0}  \right]$. Hence, in our case, we should estimate the norm of gradient of forward operator for under-sampling \ac{MRI}  and the distance between true image space and the output of the proposed optimization method, namely  $\E \left[\norm{\mbf{X}_0 -  {\text{prox}} \left(\mbf{\hat X}_0 - \lambda \nabla_{\mbf{\hat X}_0} \widehat{L}\left(\mbf{\hat X}_0,  \rho \right)  \right)}  \right]$

\paragraph{\underline{Proposed Method}} In the proposed method, namely Diffusion Proximal Projected Method, we utilize \ac{DDPM} sampling method as in Proposition \ref{prop:prop_1} incorporating with Fourier slice-based optimization in Algorithm \ref{algo:DDPM_Sampling_Proximal} to estimate conditional distribution $ p(\mbf y|\mbf{x}_t) $, yielding the reverse process at one step index $t$ as follows:
\begin{equation*}
\begin{aligned}
\mbf{\hat{x}}_0  &=\frac{1}{\sqrt{\bar \alpha_t}} \left( \mbf{x}_t + \left(1 - \bar{\alpha_t}\right) \nabla_{\mbf{x}_t} \log p\left(\mbf{x}_t \right)\right) \\
    \mbf{x}_{t-1}  &=  {\text{prox}} \left(\mbf{\hat x}_0  - \lambda \nabla_{\mbf{\hat x}_0}  \widehat{L}\left(\mbf{\hat x}_0 ,  \rho \right)  \right),
\end{aligned}
\end{equation*}
where the function $ \widehat{L}\left(\mbf{\hat x}_0, \rho \right) $ is the loss function of proposed optimization method. We will show that we can improve the approximation bound given in the Theorem \ref{thm:theorem_dppm} below. 
\begin{theorem}
\label{thm:theorem_dppm}
Suppose we have the update from proposed algorithm, namely $\textcolor{blue}{\mbf{\tilde x}_0 }= \text{prox}_{\alpha} \left( \mbf{\hat x}_0 - \lambda \nabla_{\mbf{\hat x}_0}\left(\widehat{L}\left(\mbf{\hat x}_0,  \rho \right)   \right) \right)$,  with $\mbf{\hat x}_0$ is the posterior mean given in Proposition \ref{prop:prop1} and step size $\lambda = \frac{1}{L}$ where $L$ is the Lipschitz constant of the loss function in Lemma \ref{lemma:lipschitz_loss}. Hence, we have
\begin{equation}
\card{ \E\left[p\left(\mbf{y} | \mbf{x}_0\right)\right]- p\left(\mbf{y} | \textcolor{blue}{\mbf{\tilde x}_0}\right)} \leq  \textcolor{blue}{\frac{e^{-\frac{1}{2}} }{\sqrt{\left(2\pi\right)^d\sigma^{2d + 2}}}} \underset{\mbf{x}}{\text{max}}\norm{\nabla_{\mbf{x}} \mcl{A}\left(\mbf{x}\right)}_2 \textcolor{blue}{m_2},
\end{equation}
where $\textcolor{blue}{m_2 = 2 m_1}$.
\end{theorem}
Theorem \ref{thm:theorem_dppm} shows that we can reduce the error approximation in comparison to the approximation in the Theorem \ref{thm:theorem1}, where we have the dimension parameter $d$ in the denominator instead of in the numerator. Therefore, we have a better approximation to estimate $p\left(\mbf{y} | \mbf{x}_t\right)$. %This theoretical result shows why our proposed method performs better numerical reconstruction compared to the existing diffusion model for MRI reconstruction. 
We provide the proof as well as supporting Lemma in Section \ref{sec:proof_supporting_lemma}.

As discussed in \cite[Sect. 4.2. Proximal Gradient Method]{parikh2014proximal}, the chosen range of $\lambda$ should be in  between $\lambda \in (0,\frac{1}{L}]$.  From Lemma \ref{lemma:lipschitz_loss} we have $L =5 + 2\rho \sqrt{N}$ and we can choose the step size $\lambda = \frac{1}{ \left(5 + 2\rho \sqrt{N} \right)}$ to derive the result in Theorem \ref{thm:theorem_dppm}. In our numerical results, we show that for all data we perform reconstruction with  $\lambda = 0.01$ and $\rho = 1$, which is between in the range of $\lambda$ for the image dimension plant roots $N = 128$, BRATS $N = 240$, and knee $N = 320$.
\subsection{Proximal Operator and Regularization} \label{Sect:Prox_Regul}
The implementation of the regularization function in the optimization problem can be represented as the proximal operator \cite{parikh2014proximal}. Here, we will present the proximal operator that is used in this article, namely the soft thresholding operator. Soft thresholding operator can be written as \cite[eq. 15.22]{foucart2013mathematical}.
\begin{equation}
  \label{eq: prox_soft_thres}\text{prox}_\alpha\left(\textbf{\emph X}\right)=\begin{cases}
			\frac{\textbf{\emph X}}{\card{\textbf{\emph X}}}\circ \left(\card{\textbf{\emph X}} - \alpha\right), & \text{if $\card{\textbf{\emph X}}  \geq \alpha$}\\
            0, & \text{otherwise},
		 \end{cases}
\end{equation}
where $\alpha$ is the pre-determined threshold value. It should be noted that the absolute value sign is applied element-wise for volume data.

Apart from sparsity regularization with soft thresholding operator, in this article, we also perform approximated total variation norm applied on the volumetric data $\textbf{\emph X} \in \C^{S \times N \times N}$ defined as follows \cite{barbero2010fast}
\begin{equation*}
\begin{aligned}
\norm{\textbf{\emph X}}_{\text{ATV}} &= \sum_{s = 1}^S \sum_{i = 1}^N\sum_{j = 1}^{N-1} \card{x_{s,i,j}  - x_{s, i,j+1} }^2 +  \sum_{s = 1}^S \sum_{i = 1}^{N-1}\sum_{j = 1}^N \card{x_{s,i,j} - x_{s,i+1,j}}^2 
\end{aligned}
\end{equation*}
This metric is the approximated total variation norm, since we apply squared of absolute value to the differences of each element in both axes of a matrix, i.e., for each slice $s$ we have matrix $\mbf X_s = \left(x_{i,j}\right)_s\,\text{for}\, i,j \in [N],\, s \in [S]$. We calculate this metric for all slices in volumetric data.

Here we will describe the matrix representation of approximated total variation norm. We can define the matrix operator to measure the difference of elements for a vector as follows
\begin{equation}
\label{eq:deriv_matrix}
   \mbf{D} = \begin{pmatrix}
-1 & 1 & 0 & 0 & \hdots & 0\\
0 & -1 & 1 & 0 & \hdots & 0\\
0 &  0 & -1 & 1 & \hdots & 0\\ 
\vdots & \vdots & \vdots & \vdots & \vdots & \vdots \\
0 & 0 & \hdots & \hdots & -1 & 1\\
\end{pmatrix} \in \R^{N-1 \times N}.
\end{equation}
It can be seen that for any vector multiplied with  \eqref{eq:deriv_matrix}, we get another vector with a new dimension $N-1$ with each element measure the difference between adjacent position. If we flatten the slice matrix $\mbf{\tilde x}_s = \text{vec}\left(\mbf{X}_s\right) \in \C^{N^2}$, we can write another matrix operator to measure the differences in both axes row and column of a matrix as follows:
\begin{equation}
   \mbf{B} = \begin{pmatrix}
\mbf{I}\,\otimes \mbf{D}\\
\mbf{D} \otimes \mbf{I}\\
\end{pmatrix} \in \R^{2(N-1)N \times N^2},  
\end{equation}
where the structure of block matrix $\mbf B$ can be written as
\begin{equation}
\label{eq:deriv_matrix_2}
   \mbf{B} = \begin{pmatrix}
\mbf{D} &  0  &  \hdots & \hdots &\hdots & 0\\
0 &  \mbf D &  \hdots & \hdots &\hdots & 0\\
\vdots &  0 &  \mbf D  & \hdots &\hdots & 0\\
\vdots&  \hdots  & \vdots &\hdots & \ddots & \vdots\\
0&  \hdots & 0 & \hdots &\hdots & \mbf D\\
-\mbf{I}&  \mbf{I} & 0 & \hdots &\hdots & \mbf 0\\
0&  -\mbf{I} & \mbf{I} & \hdots & \hdots & \mbf 0\\
\vdots &  0 & -\mbf{I} &\mbf{I}& \hdots & \vdots\\
\vdots &  \vdots & \vdots &\vdots & \hdots & \vdots\\
\vdots &  \vdots & \vdots &\vdots &  -\mbf{I} &\mbf{I}&\\
\end{pmatrix} \in \R^{2(N-1)N \times N^2}
\end{equation}
The matrix \eqref{eq:deriv_matrix_2} represents the calculation of both row and column axes of the original matrix slice, in vector style. In addition, if we consider flattening all volumetric data, the approximated total variation norm can be rewritten as
\[
\underbrace{\begin{pmatrix}
\mbf{\tilde b}_1 \\
\vdots\\
\mbf{\tilde b}_S \end{pmatrix}}_{\mbf{\tilde b}} = \underbrace{\begin{pmatrix}
\mbf{B} &\hdots &0 \\
\vdots & \ddots & \vdots \\
0& \hdots & \mbf{B}
\end{pmatrix}}_{\mbf{\tilde B} \in \R^{2S(N-1)N \times SN^2}}
\underbrace{\begin{pmatrix}
\mbf{\tilde x}_1 \in \C^{N^2}\\
\vdots\\
\mbf{\tilde x}_S \in \C^{N^2}\end{pmatrix}}_{\mbf{\tilde x}}\in \C^{SN^2},
\]
Hence, the approximated total variation norm for volumetric data is equivalent to the $\ell_2-$norm of its flattening version
\begin{equation}
\label{eq:atv}
\norm{\textbf{\emph X}}_{\text{ATV}} = \norm{\mbf{\tilde b}}_2^2 = \norm{\mbf{\tilde B}\mbf{\tilde x}}_2^2  
\end{equation}
It should be noted that here we introduce the matrix $\mbf{\tilde B}$ as the operator to calculate the difference of elements in the volumetric data. It is important to estimate the eigenvalue of this matrix for convergence analysis. The result is presented in the following proposition
\begin{proposition}
\label{prop:prop_2}
    The maximum eigenvalue of the matrix $\mbf{\tilde B}^H\mbf{\tilde B}$ is $4$.
\end{proposition}
\begin{proof}
    We can estimate the spectral norm of matrix $\mbf{\tilde B}$, $\norm{\mbf{\tilde B}}^2 = {\text{eig}_{max}\left(\mbf{\tilde B}^H \mbf{\tilde B} \right)}$. The gram matrix $\mbf{\tilde B}^H \mbf{\tilde B}$ can be written as
    \begin{equation}
        \mbf{\tilde B}^H \mbf{\tilde B} = \begin{pmatrix}
\mbf{B}^H\mbf{B} &\hdots &0 \\
\vdots & \ddots & \vdots \\
0& \hdots & \mbf{B}^H\mbf{B}
\end{pmatrix}
    \end{equation}
Since the matrix is a block diagonal matrix, it is enough to estimate the maximum eigenvalue for 
\begin{equation}
\begin{aligned}
    \mbf{\tilde B}^H \mbf{\tilde B} &\stackrel{\text{(a)}}{=}  \left(\mbf{I}^H \otimes \mbf{D}^H\right) \left(\mbf{I} \otimes \mbf{D}\right) +  \left( \mbf{D}^H \otimes\mbf{I}^H\right)\left( \mbf{D} \otimes\mbf{I} \right)\\
    &\stackrel{\text{(b)}}{=} \left(\mbf{I} \otimes \mbf{D}^H \mbf{D} +    \mbf{D}^H \mbf{D} \otimes \mbf{I} \right),
\end{aligned}
\end{equation}
where the equality of (a) and (b) are given by the property of conjugate transpose Kronecker product and the mixed-product property of Kronecker product and matrix product, respectively. The product of $\mbf{D}^H \mbf{D}$ has tridiagonal structure as follows
\begin{equation*}
    \mbf{D}^H \mbf{D} = \begin{pmatrix}
        2& -1 & 0 & \hdots & \hdots& \hdots \\
        -1& 2 & -1 & \hdots& \hdots & \hdots \\
        0& -1 & 2 & -1 & \hdots& \hdots \\
        \vdots& \hdots & -1 & 2 & -1& \hdots \\
         \vdots& \hdots & \hdots & \hdots & \ddots & \hdots \\
          \vdots& \hdots & \hdots & \hdots & -1 & 2 \\ 
    \end{pmatrix} \R^{N \times N},
\end{equation*}
where it is well-known, for instance in \cite{barbero2010fast, noschese2013tridiagonal, kulkarni1999eigenvalues}, eigenvalues of $\mbf{D}^H \mbf{D}$ is given by
$$
\omega_i = 2 - 2 \cos\left(\frac{i\pi}{N
}\right) \,\text{for}\, i \in [N-1].
$$
The maximum is then $2$.  Now, having the property of the eigenvalue, we can estimate the eigenvalue of
$$
\mbf{\tilde B}^H \mbf{\tilde B}= \mbf{I} \otimes \mbf{D}^H \mbf{D} +    \mbf{D}^H \mbf{D} \otimes \mbf{I} $$
In fact, from \cite[Chap 5. ex. 39]{merris1997multilinear}, the eigenvalue is given by 
$\omega_i + \omega_j$ for $i,j \in [N-1]$. In other words, the list of eigenvalues consists of the sum of all possible combinations of the eigenvalues of $\mbf{D}^H \mbf{D}$. Hence, the maximum eigenvalue of $ \mbf{\tilde B}^H \mbf{\tilde B} $ is given by $4$
\end{proof}
\subsection{Fourier slice theorem} \label{sec:FourierSlice}
We follow the definition and presentation of the Fourier slice method as given in \cite{bracewell1990numerical, bracewell1956strip}. Suppose we have 2D function $p(x,y)$, the projection can be written as
\begin{equation*}
p(x) = \int_{-\infty}^{\infty} p(x,y) dy
\end{equation*}
Now observe the 2D Fourier transform $\widehat{p}(k_x,k_y) = \mcl{F}_{2D} \left( p(x,y)\right)$
\begin{equation*}
\widehat{p}(k_x,k_y) ) = \int_{-\infty}^{\infty} \int_{-\infty}^{\infty} p(x,y) e^{-2\pi(x k_x + y k_y)} dx dy
\end{equation*}
Focusing on the slice at the center frequency at $y-$axis, i.e.,  $k_y = 0$, we have
\begin{equation*}
\begin{aligned}
\widehat{p}(k_x,0)  &= \int_{-\infty}^{\infty} \int_{-\infty}^{\infty} p(x,y) dy \, e^{-2\pi x k_x} dx = \int_{-\infty}^{\infty} p(x) e^{-2\pi x k_x} dx = \mcl{F}_{1D} \left( p(x)\right)
\end{aligned}
\end{equation*}
This is a 1D Fourier transform on the projection. Additionally, the projection in the discrete setting is the summation on the one axis. 
Suppose we have square matrices representing the k-space and image space data for each slice $\mbf{Y}_s \in \C^{N \times N}$ and $\mbf{X}_s \in \C^{N \times N}$ for $s \in [S]$, respectively. The relation of sliced k-space on the zero frequency at $y-$axis, i.e., ${\mbf{y}}_s^{k_x} = \mbf{Y}_s \vert_{\left(k_y = 0\right)} \in \C^{N}$ and the image space can be written as
$$ 
{\mbf{y}}_s^{k_x} = \mcl{F}_{1D}\left(\mcl{P}_{x}\left(\mbf{X}\right)\right) \in \C^N,
$$
where $\mcl{P}_{x}\left(\mbf{X}_s\right) \in \C^{N}$ is a vector after summing the matrix on $y-$axis, so we only have dimension on $x-$axis. We can write in discrete case as
\begin{equation}
\footnotesize
\begin{aligned}
\mcl{P}_{x}\left(\mbf{X}\right) &= \left( \sum_{j = 1}^{N} x_{1,j},  \sum_{j = 1}^{N} x_{2,j},\hdots, \sum_{j = 1}^{N} x_{N,j} \right)^T \in \C^{N} \\&\leq \sqrt{N} \left(\sqrt{\sum_{j = 1}^{N} \card{x_{1,j}}^2}, \sqrt{\sum_{j = 1}^{N} \card{x_{2,j}}^2}, \hdots, \sqrt{\sum_{j = 1}^{N} \card{x_{N,j}}^2} \right)^T \in \C^N
\end{aligned}
\end{equation}
The inequality follows from Cauchy-Schwarz inequality.
\subsection{Matrix-Vector Representation of Fourier Transforms and Optimization Problem}\label{sec:MatrixVector}
In this section, we simplify the notation that will be useful for the analysis of the optimization part in Diffusion Proximal Projection Method \eqref{eq:opt}. The reformulation in this section is only used for analysis, not the implementation. Since Fourier transform is a linear operator applied on matrix and vector space, the operation with Fourier transform can be represented by matrix-vector product. Suppose we have a vector $\mbf{x} \in  \R^N$, then the one-dimensional Fourier transform can be written as
$$
\mcl{F}_{1D}\left( \mbf{x} \right) = \mbf{F}_{1D} \mbf{x},
$$
where the matrix $\mbf{F}_{1D} \in \C^{N \times N}$ is the matrix representation of one-dimensional Fourier transform.

Additionally, if we have a matrix $\mbf{X} \in \R^{N \times N}$ the two-dimensional Fourier transform can be written as
$$
\text{vec}\left( \mcl{F}_{2D}\left( \mbf{X} \right) \right) = \mbf{F}_{2D} \text{vec}\left( \mbf{X}\right),
$$
where $\text{vec}: \R^{N \times N} \rightarrow \R^{N^2}$, is a function to flatten the matrix into vector and $\mbf{F}_{2D} = \mbf{F}_{1D} \otimes \mbf{F}_{1D} \in   \C^{N^2\times N^2}$ is the representation of two-dimensional Fourier matrix by applying Kronecker product $\otimes$ on two of one-dimensional Fourier matrices \cite[eq.5.68]{jain1989fundamentals}. In this article, we follow the definition of unitary property of Fourier matrices, i.e., $\mbf{F}_{2D}^H \mbf{F}_{2D} = \mbf{I} \in \R^{N^2 \times N^2}$ and $\mbf{F}_{1D}^H \mbf{F}_{1D} = \mbf{I} \in \R^{N \times N}$.

The concept of element-wise or Hadamard product of two matrices $\mbf{Y} \circ \mbf{X}$  can be written as 
$$
\text{vec}\left(\mbf{X} \circ \mbf{Y}\right) = \text{diag}\left(\text{vec}\left(\mbf{X}\right)\right) \text{vec}\left(\mbf{Y}\right) \in \R^{N^2},
$$ 
where the $\text{diag}\left(\text{vec}\left(\mbf{X}\right)\right) $ is a diagonal matrix which contains vectorization of matrix $\mbf{X}$ on the main diagonal element.
It should be noted that the element-wise or Hadamard product has a commutative property, hence, swapping the position preserves the result.

We recall the model for under-sampled k-space $\hat{\mbf{Y}}$ with the undersampling or masking operator $\mbf{M} \in \R^{N \times N}$, i.e., matrix with one and zero elements, with the MR image, i.e., the image of interest $\mbf{X}$:
\begin{equation}
\label{eq:forward_2d}
\hat{\mbf{Y}}_s = \mbf{M} \circ \left( \mcl{F}_{2D}\left( \mbf{X}_s \right)\right)\,\text{for}\, s \in [S]    
\end{equation}
Suppose vector $\mbf{\tilde{y}}_s = \text{vec}\left({\mbf{\hat Y}_s} \right) \in \C^{N^2}$ and vector $\mbf{\tilde{x}}_s = \text{vec}\left({\mbf{X}}_s \right) \in \C^{N^2}$ are the vectorization or flattening version of under-sampled k-space at specific slice $\hat{\mbf{Y}}_s$ and image space $\mbf{X}_s$, respectively. Additionally, the masking operator and two-dimensional Fourier transform can be written as a single matrix 
$$\mbf{A}  := \text{diag}\left( \text{vec}\left(\mbf{M} \right)\right)\mbf{F}_{2D} \in \C^{N^2 \times N^2}.$$Therefore, we can write  the equivalent formulation of \eqref{eq:forward_2d} as
\begin{equation}
\label{eq:matrix_forward_model}
\mbf{\tilde{y}} = \underbrace{\left(\mbf{I} \otimes \mbf{A}\right)}_{\mbf{\tilde A}}    \mbf{\tilde{x}} \in \C^{SN^2}, 
\end{equation}
where we stack the vectorization of each slice k-space $\mbf{\tilde y}_s \in \C^{N^2}$ and the image space  $\mbf{\tilde x}_s \in \C^{N^2}$ into a  new vector with dimension $SN^2$. In other words, $\mbf{\tilde y}$ and $\mbf{\tilde x}$ are vectorizations of volumetric data.
\[
\underbrace{\begin{pmatrix}
\mbf{\tilde y}_1 \\
\vdots\\
\mbf{\tilde y}_S \end{pmatrix}}_{\mbf{\tilde y}} = \underbrace{\begin{pmatrix}
\mbf{A} &\hdots &0 \\
\vdots & \ddots & \vdots \\
0& \hdots & \mbf{A}
\end{pmatrix}}_{\mbf{\tilde A} \in \C^{SN^2 \times SN^2}} \underbrace{\begin{pmatrix}
\mbf{\tilde x}_1 \in \C^{N^2} \\
\vdots\\
\mbf{\tilde x}_S \in \C^{N^2}\end{pmatrix}}_{\mbf{\tilde x}}\in \C^{SN^2}
\]
Furthermore, let us write matrix representation of one-dimensional Fourier transform and sliced undersampling matrix $\mbf{A}_y = \text{diag}\left(\mbf{m}^{k_y}\right) \mbf{F}_{1D} \in \C^{N \times N}$ and $\mbf{A}_x = \text{diag}\left(\mbf{m}^{k_x}\right) \mbf{F}_{1D} \in \C^{N \times N}$. Thereby, the projection constraint with the projection on $y-$axis and $x-$axis, namely
\begin{equation*}
\begin{aligned}
\hat{\mbf{y}}_s^{k_y} &= \mbf{m}^{k_y} \circ \mcl{F}_{1D}\left( \mcl{P}_{y} \left(\mbf{X}_s\right) \right) \quad \text{and} \quad
\hat{\mbf{y}}_s^{k_x} &= \mbf{m}^{k_x} \circ \mcl{F}_{1D}\left( \mcl{P}_{x} \left(\mbf{X}_s\right) \right) \, \text{for} \, s \in [S],
\end{aligned}
\end{equation*}
can also be written in the matrix-vector form, as follows: 
\begin{equation}
\label{eq:matrix_forward_model_constraint}
\hat{\mbf{y}}^{k_y} = \underbrace{\left(\mbf{I} \otimes \mbf{A}_y \right)}_{\mbf{\tilde A}_y} \nu_y\left(\mbf{\tilde x}\right) \in \C^{SN}\quad \text{and} \quad
\hat{\mbf{y}}^{k_x} = \underbrace{\left(\mbf{I} \otimes \mbf{A}_x \right)}_{\mbf{\tilde A}_x}\nu_x\left(\mbf{\tilde x}\right) \in \C^{SN},
\end{equation}
where the function $\nu : \C^{SN^2} \rightarrow \C^{SN}$ maps the flattening of three-dimensional data into a vector projection for each slice and stack into a new vector. The visualization can be written, for instance for $\hat{\mbf{y}}^{k_y} $
\[
\underbrace{\begin{pmatrix}
\mbf{\hat y}^{k_y}_1 \\
\vdots\\
\mbf{\hat y}^{k_y}_S \end{pmatrix}}_{\mbf{\hat y}^{k_y}} = \underbrace{\begin{pmatrix}
\mbf{A}_y &\hdots &0 \\
\vdots & \ddots & \vdots \\
0& \hdots & \mbf{A}_y
\end{pmatrix}}_{\mbf{\tilde A}_y \in \C^{SN \times SN}} \underbrace{\begin{pmatrix}
\mcl{P}_{y}\left(\mbf{X}_1 \right)\in \C^N \\
\vdots\\
\mcl{P}_{y}\left(\mbf{X}_S \right)\in \C^N\end{pmatrix}}_{\nu_y\left(\mbf{\tilde x}\right)}\in \C^{SN}.
\]
The visualization for $\hat{\mbf{y}}^{k_x} $ should follow directly by applying the same definition on $x-$axis. Since the projection is linear operator, we can write $\nu_y\left(\mbf{\tilde x_0}\right) - \nu_y\left(\mbf{\tilde z_0}\right) = \nu_y\left(\mbf{\tilde x_0} - \mbf{\tilde z_0}\right)$.  Additionally,
we have 
\begin{equation}
\begin{aligned}
\label{eq:upper_bound_proj}
\norm{\nu_y\left(\mbf{\tilde x}\right)}_2 &= \sqrt{\sum_{s=1}^S \norm{\mcl{P}_{y}\left(\mbf{X}_s \right)}_2^2} \leq \sqrt{N \sum_{s=1}^S \sum_{i = 1}^N \sum_{j = 1}^N \card{x_{sij}}^2} = \sqrt{N} \norm{\mbf{\tilde x}}_2.
\end{aligned}
\end{equation}
The structure of eigenvalue of matrices $\mbf{\tilde A} \in \C^{SN^2 \times SN^2}$, $\mbf{\tilde A}_y \in \C^{SN \times SN}$, and $\mbf{\tilde A}_x \in \C^{SN \times SN}$ are important later for the analysis of Lipschitz constant. Here, we provide the result in the following proposition
\begin{proposition}
\label{prop:prop_1}
    The maximum eigenvalue of the matrix $\mbf{\tilde A}^H\mbf{\tilde A} \in \C^{SN^2 \times SN^2}$, the matrix $\mbf{\tilde A}_y^H\mbf{\tilde A}_y \in \C^{SN \times SN}$, as well as the matrix $\mbf{\tilde A}_x^H\mbf{\tilde A}_x \in \C^{SN \times SN}$ is $1$.
\end{proposition}
\begin{proof}
    The spectral norm of the matrix $\mbf{\tilde A} $ is used to estimate the maximum eigenvalue and can be written as $\lVert\mbf{\tilde A}\rVert^2 = \lVert\mbf{\tilde A}^H\mbf{\tilde A}\rVert =  {\text{eig}_\text{max}\left(\mbf{\tilde A}^H\mbf{\tilde A}  \right)}$. First, we will calculate the matrix product
    \begin{equation}
    \begin{aligned}
        \mbf{\tilde A}^H\mbf{\tilde A} &= \left(\mbf{I} \otimes \mbf{A} \right)^H\left(\mbf{I} \otimes \mbf{A} \right)  \stackrel{\text{(a)}}{=}  \left(\mbf{I}^H \otimes \mbf{A}^H \right)\left(\mbf{I} \otimes \mbf{A} \right) \\
        &\stackrel{\text{(b)}}{=} \left(\mbf{I}^H\mbf{I} \otimes \mbf{A}^H\mbf{A} \right)\\
      %  &=  \mbf I \otimes \left(\mbf{F}_{2D}^H\text{diag}\left( \text{vec}\left(\mbf{M} \right)\right)\mbf{F}_{2D} \right)
    \end{aligned}
    \end{equation}
    The equality (a) is the property of conjugate transpose for Kronecker product. The equality (b) is derived from the mixed-product property between Kronecker and matrix product. The last equation  $\left(\mbf{I}  \otimes \mbf{A}^H\mbf{A} \right) \in \C^{SN^2 \times SN^2}$ is a block diagonal matrix, where the matrix in the diagonal is circulant matrix \cite[eq 5.85]{jain1989fundamentals}, namely $\mbf{  A}^H\mbf{  A} = \mbf{F}_{2D}^H\text{diag}\left( \text{vec}\left(\mbf{M} \right)\right)\mbf{F}_{2D}$. Therefore, the maximum eigenvalue of matrix $\mbf{\tilde A}^H\mbf{\tilde A}$ is the maximum eigenvalue of the circulant matrix, where in this case, since we have the diagonal element as flattening undersampling or masking matrix with element between $0$ and $1$. we have maximum eigenvalue $1$. Similar approach  can be adopted for both matrices   $\mbf{\tilde A}_y \in \C^{SN \times SN}$, and $\mbf{\tilde A}_x \in \C^{SN \times SN}$.
\end{proof}
The result from Proposition \ref{prop:prop_1} will be used later to derive the condition on the Lipschitz constant of the loss function to get the upper bound of the approximation error.
%\text{diag}\left( \text{vec}\left(\mbf{M} \right)\right)\mbf{F}_{2D}
Taking the matrix-vector representation of Fourier transform and the function for regularization from Section \ref{Sect:Prox_Regul}, we can use the matrix-vector representation in \eqref{eq:matrix_forward_model}, \eqref{eq:matrix_forward_model_constraint}, and \eqref{eq:atv} to write the equivalence of the optimization problem in the main article \eqref{eq:opt} as matrix-vector fashion in the following
\begin{equation}
\begin{aligned}
\label{eq:opt_matrix}
& \underset{\mbf{\tilde x}\in \C^{SN^2}}{\text{minimize}}
& &  \norm{\mbf{\tilde y} - \mbf{\tilde A} \mbf{\tilde x}}_2^2 + \left(\alpha \norm{\mbf{\tilde x}}_1 + \norm{\mbf{\tilde B}\mbf{\tilde x}}_2^2   \right) \\
& \text{subject to}
& &  \hat{\mbf{y}}^{k_y} =  \mbf{\tilde A}_y \nu_y\left(\mbf{\tilde x}\right)\\
&&& \hat{\mbf{y}}^{k_x} =  \mbf{\tilde A}_x \nu_x\left(\mbf{\tilde x}\right)\\,
\end{aligned}
\end{equation}
Thereby, loss function for three-dimensional data in terms of its flattening version, i.e., $\mbf{\tilde x} \in \C^{SN^2}$, $ \widehat{L}\left(\mbf{\tilde x}, \rho \right) $ is given in the following.
\begin{equation}
\footnotesize
\begin{aligned}
\label{eq:loss_equivalence}
\widehat{L}\left(\mbf{\tilde x}, \rho \right) &= \frac{1}{2}\norm{\mbf{\tilde{y}}- \mbf{\tilde A} \mbf{\tilde x} }_2^2  + \frac{\rho}{2}\norm{\hat{\mbf{y}}^{k_y} - \mbf{\tilde A}_y \nu_y \left(\mbf{\tilde x}\right)}_2^2 + \frac{\rho}{2}\norm{\hat{\mbf{y}}^{k_x} - \mbf{\tilde A}_x \nu_x\left(\mbf{\tilde x}\right)}_2^2 + \frac{1}{2} \norm{\mbf{\tilde B}\mbf{\tilde x}}_2^2 
\end{aligned}
\end{equation}
%+ \rho\left(\norm{ \hat{\mbf{y}}_s^{k_y} - \mbf{m}^{k_y} \circ \mcl{F}_{1D}\left( \mcl{P}_{zy} \left(\mbf{X}_s\right)\right)}_2^2 + \norm{ \hat{\mbf{y}}_s^{k_x} -  \mbf{m}^{k_x} \circ \mcl{F}_{1D}\left( \mcl{P}_{zx} \left(\mbf{X}_s\right)\right)}_2^2\right)
Note that, the Frobenius norm in the original formulation is replaced by Euclidean or $\ell_2$-norm because we vectorized or flattened each slice matrix. Hence, the total update for the algorithm for matrix-vector representation can be written as
\begin{equation}
\label{eq:proximal_matrix_vector}
    \mbf{\tilde x}^{\left(i\right)} =  {\text{prox}_{\alpha}} \left(\mbf{\tilde x}^{\left(i-1\right)} - \lambda \nabla_{\mbf{\tilde x}^{\left(i-1\right)}} \widehat{L}\left(\mbf{\tilde x}^{\left(i-1\right)},  \rho \right)  \right) \in \C^{SN^2},
\end{equation}
The proximal in this case is the soft thresholding operator in \eqref{eq: prox_soft_thres}. 

\subsection{Supporting Lemmas and Proof of Main Theorem}\label{sec:proof_supporting_lemma}
Before we state the result, here we will discuss the necessary tools to derive the result. Since both conditional density functions $p\left(\mbf{y}|\mbf{x}_t \right)$ and $p\left(\mbf{y}|\mbf{\hat x}_0 \right)$ are Gaussian. We first state the Lipschitz condition of the Gaussian probability density function in the following Lemma.
\begin{lemma}
\label{lemma:multivar_gauss}
    Suppose we have an isotropic multivariate Gaussian probability density function  with mean $\bs \mu$ and variance $\sigma^2 \mbf{I}$. Hence, for all input $\mbf{x}, \mbf{y} \in \R^d$ we have 
\begin{equation}
\norm{p\left(\mbf x\right) - p\left(\mbf y\right)}_2 \leq L \norm{\mbf x - \mbf y}_2,
\end{equation}
where the constant $L =  \frac{e^{-\frac{1}{2}} }{\sqrt{\left(2\pi\right)^d\sigma^{2d + 2}}} $
\end{lemma}
\begin{proof}
For a vector random variable $\mbf{n} \in \R^d \sim \mcl{N}\left(\bs \mu, \sigma^2 \mbf I \right) $, we have probability density function
$$
p\left(\mbf{n}\right) = \frac{1}{\sqrt{(2\pi \sigma^2)^d}} \exp\left(- \frac{\norm{\mbf n - \bs \mu}^2_2}{2\sigma^2} \right)
$$
It should be noted that this function maps from the input vector into scalar since the norm transforms the vector into a scalar. From the mean value theorem, we have
$$
\norm{p\left(\mbf x\right) - p\left(\mbf y\right)}_2 \leq \underset{\forall \mbf{z} \in \R^d}{\text{max}} \norm{\nabla_{\mbf z} p(\mbf z)}_2 \norm{\mbf x - \mbf y}_2,
$$
where the maximum $\underset{\forall \mbf{z} \in \R^d}{\text{max}} \norm{\nabla_{\mbf z} p(\mbf z)}_2$ is similar to find maximum norm of the function $p(.)$ for all possible inputs. For multivariate case, the $\norm{\nabla_{\mbf z} p(\mbf z)}_2$ can be written as
$$
\norm{\nabla_{\mbf z} p(\mbf z)}_2 = \frac{1}{\sqrt{\left(2\pi\sigma^2\right)^d}}  \exp\left(-\frac{\norm{\mbf z - \bs \mu}^2_2}{2\sigma^2} \right)\frac{1}{\sigma^2}\norm{\mbf z - \bs \mu}_2
$$
Additionally, let us write scalar $a = \norm{\mbf z - \bs \mu}_2$. Maximizing the function with respect to $\mbf z$ is equivalent to maximizing the scalar $a$. Therefore, it is similar to what we have in the univariate case, where we have

$$
\underset{\forall a \in \R}{\text{max}} \card{\frac{a}{\sigma^2} p(a)} = \frac{e^{-\frac{a^2}{2\sigma^2}}}{\sqrt{\left(2\pi\sigma^2\right)^d}} \frac{a}{\sigma^2}
$$
The maximum can be analyzed by taking a derivative so we have
$$
\frac{\mrm{d}}{\mrm d a} \frac{a}{\sigma^2} p(a) = \frac{\left(\frac{1}{\sigma^2} - \left(\frac{a}{\sigma^2}\right)^2 \right)e^{-\frac{a^2}{2\sigma^2}}}{\sqrt{\left(2\pi\sigma^2\right)^d}},
$$
where the maximum is achieved by taking the derivative equal to zero to get $a = \pm \sigma$. Therefore, we have 
$$\underset{\forall \mbf{z} \in \R^d}{\text{max}} \norm{\nabla_{\mbf z} p(\mbf z)}_2 \leq \frac{e^{-\frac{1}{2}} }{\sqrt{\left(2\pi\right)^d\sigma^{2d + 2}}}= L  $$
\end{proof}
 
In the proposed method, given in Algorithm \ref{algo:DDPM_Sampling_Proximal}, we incorporate the proximal method \eqref{eq:proximal_matrix_vector} to solve the optimization problem in \eqref{eq:opt} or its matrix-vector equivalent \eqref{eq:opt_matrix}.  We first present the property of proximal operators given in \cite{parikh2014proximal, garrigos2023handbook}. 
\textcolor{black}{First}, as discussed in \cite[Lemma 8.17]{garrigos2023handbook}, the proximal operator does not change the optimality.
\begin{lemma}[Lemma 8.17 \cite{garrigos2023handbook}, Sec.2.3 \cite{parikh2014proximal}]
\label{lemma:prox_preserve}
Suppose we have functions $\widehat{L} + g$, where $\widehat{L}$ is the loss function and convex differentiable and $g$ is the lower semi continues for regularization. If $\mbf{x}_0 \in $ \text{arg min}$\left(\widehat{L} + g\right)$, then
$$
\mbf{x}_0  = {\text{prox}  \left(\mbf{x}_0 - \lambda \nabla_{\mbf{x}_0} \widehat{L}\left(\mbf{x}_0,  \rho \right)  \right)},  
$$
for $\lambda > 0$
\end{lemma}
This property shows that if we apply the proximal method combined with gradient update to the optimal solution, we still have the optimal solution specific to the loss function we consider in the proposed optimization method. \textcolor{black}{Additional property} for proximal function is that it is non-expansive as presented in \cite[Lemma 8.16]{garrigos2023handbook}, as follows:
\begin{lemma}[Lemma 8.16\cite{garrigos2023handbook}, Fixed Point Algorithm p.131 \cite{parikh2014proximal}]
\label{lemma:prox_non_expansive}
The proximal operator is $1-$ Lipschitz and non-expansive as follows
\begin{equation}
\norm{\text{prox}\left(\mbf{x}_0 \right) - \text{prox} \left(\mbf{\hat{x}}_0\right)}_2 \leq \norm{ \mbf{x}_0 - \mbf{\hat{x}}_0}_2
\end{equation}
\end{lemma}

Since we perform gradient of the loss function, we will discuss the property of Lipschitz constant of the loss function by using the property of Lipschitz constant in \cite[Definition 2.24]{garrigos2023handbook}, as follows: 
\begin{definition}
\label{definition:lipschitz}
Let $\mcl{F}: \C^D\rightarrow \C^D$, and $L > 0$. The differentiable function $\mcl F$ is {L-Lipschitz} if $ \forall \mbf{x}, \mbf{z} \in \C^D, \norm{\nabla_{\mbf{z}} \mcl{F}\left(\mbf z \right) - \nabla_{\mbf{x}} \mcl{F}\left(\mbf x \right)}_2 \leq L \norm{\mbf{z} - \mbf{x}}_2$
\end{definition}
%\begin{equation}
%\norm{\nabla \mcl{F}\left(\mbf{ X}_0  \right) - \nabla \mcl{F}\left(\mbf{\hat X}_0  \right)} \leq L \norm{\mbf{ X}_0  - \mbf{ \hat X}_0 }
%\end{equation} 
In general, if we can find minimum constant $L$ such that equation in Definition \ref{definition:lipschitz} holds, we can say that the function $\mcl{F}$ is $L-$ Lipschitz. 
\begin{lemma}
\label{lemma:lipschitz_loss}
    Given the loss function $\widehat{L}\left(\mbf{x}_0,  \rho \right)$ of the proposed algorithm in \eqref{eq:loss_equivalence}, then we have
    $$\norm{\nabla_{\mbf{x}_0} \left(\widehat{L}\left(\mbf{x}_0,  \rho \right)  \right) - \nabla_{\mbf{z}_0} \left(\widehat{L}\left(\mbf{z}_0,  \rho \right)  \right)}_2 \leq L \norm{\mbf{x}_0 - \mbf{z}_0}_2,
    $$
    where $L = 5 + 2\rho \sqrt{N}$.
\end{lemma}

\begin{proof} 
The gradient of the loss function in \eqref{eq:loss_equivalence}, $\nabla_{\mbf{\tilde x}} \left(\widehat{L}\left(\mbf{\tilde x}, \rho \right)  \right)$, can be written as
\begin{equation}
\begin{aligned} 
\nabla_{\mbf{\tilde x}}\left(\widehat{L}\left(\mbf{\tilde x}, \rho \right)\right) &= -\mbf{\tilde A}^H\left(\mbf{\tilde{y}}- \mbf{\tilde A} \mbf{\tilde x} \right)  - {\rho}\mbf{\tilde A}_y^H \left(\hat{\mbf{y}}^{k_y} - \mbf{\tilde A}_y \nu_y \left(\mbf{\tilde x}\right)\right) \\
&- {\rho}\mbf{\tilde A}_x^H\left(\hat{\mbf{y}}^{k_x} - \mbf{\tilde A}_x \nu_x\left(\mbf{\tilde x}\right)\right) +  \mbf{\tilde B}^H\mbf{\tilde B}\mbf{\tilde x} 
\end{aligned}
\end{equation}
Then we can check the Lipschitz constant for the function  $ \widehat{L}\left(\mbf{x}, \rho \right) $. Suppose we have input for the gradient of loss function, namely $\mbf{x}_0 , \mbf{z}_0 $, then we have 
\begin{equation}
\footnotesize
\begin{aligned}
\begin{split} 
\norm{\nabla_{\mbf{x}_0 } \widehat{L}\left(\mbf{x}_0 , \rho \right) - \nabla_{\mbf{ z}_0 } \widehat{L}\left(\mbf{z}_0 , \rho \right)}_2 &= \lVert\mbf{\tilde A}^H\mbf{\tilde A} \left(\mbf{x}_0  - \mbf{z}_0  \right)+ \rho\mbf{\tilde A}_y^H\mbf{\tilde A}_y \left(\nu_y\left(\mbf{x}_0 \right) - \nu_y\left(\mbf{z}_0 \right)  \right) \\&+  \rho\mbf{\tilde A}_x^H\mbf{\tilde A}_x \left(\nu_{x}\left(\mbf{x}_0 \right) - \nu_{x}\left(\mbf{z}_0 \right) \right) + \mbf{\tilde B}^H\mbf{\tilde B}\left(\mbf{x}_0 - \mbf{z}_0\right)   \rVert_2 \\
&\stackrel{\text{(a)}}{\leq} \lVert\mbf{\tilde A}^H\mbf{\tilde A} \left(\mbf{x}_0  - \mbf{z}_0  \right)\rVert_2 + \rho\lVert\mbf{\tilde A}_y^H\mbf{\tilde A}_y \left(\nu_y\left(\mbf{x}_0 \right) - \nu_y\left(\mbf{z}_0 \right)  \right)\rVert_2 \\&+  \rho\lVert\mbf{\tilde A}_x^H\mbf{\tilde A}_x \left(\nu_{x}\left(\mbf{x}_0 \right) - \nu_{x}\left(\mbf{z}_0 \right) \right) \rVert_2+ \lVert\mbf{\tilde B}^H\mbf{\tilde B}\left(\mbf{x}_0 - \mbf{z}_0\right)   \rVert_2  \\
\end{split}
\end{aligned}
\end{equation}
The inequality (a) follows from the property of triangle inequality for norm. Here, we want to bound each norm separately. From Proposition \ref{prop:prop_1}, we know that the spectral norm $\norm{\mbf{\tilde A}^H\mbf{\tilde A}}$, $\norm{\mbf{\tilde A}_y^H\mbf{\tilde A}_y}$, and $\norm{\mbf{\tilde A}_x^H\mbf{\tilde A}_x}$ are equal to $1$. Additionally, from Proposition \ref{prop:prop_2} we have spectral norm $\norm{\mbf{\tilde B}^H\mbf{\tilde B}} = 4$. Hence, the upper bound can be written as
\begin{equation}
\footnotesize
\begin{aligned}
\begin{split} 
\norm{\nabla_{\mbf{x}_0 } \widehat{L}\left(\mbf{x}_0 , \rho \right) - \nabla_{\mbf{ z}_0 } \widehat{L}\left(\mbf{z}_0 , \rho \right)}_2 
&\stackrel{\text{(a)}}{\leq}  5\lVert\mbf{x}_0  - \mbf{z}_0\rVert_2 + \rho\lVert\nu_y\left(\mbf{x}_0 - \mbf{z}_0 \right)\rVert_2 + \rho\lVert\nu_x\left(\mbf{x}_0 - \mbf{z}_0 \right)\rVert_2\\
&\stackrel{\text{(b)}}{\leq}   5\lVert\mbf{x}_0  - \mbf{z}_0\rVert_2 + 2\sqrt{N}\rho\lVert\mbf{x}_0 - \mbf{z}_0 \rVert_2 \\& = \left(5 + 2\rho \sqrt{N} \right)\lVert\mbf{x}_0 - \mbf{z}_0\rVert_2 
\end{split}
\end{aligned}
\end{equation}
where the first inequality (a) is derived by the result on the spectral norm of the matrix given in Proposition  \ref{prop:prop_1}, Proposition \ref{prop:prop_2}, as well as by using the linear property of the projection, i.e., $\nu\left(\mbf{z}\right) - \nu\left(\mbf{x}\right)=\nu\left(\mbf{z} - \mbf{x}\right)$. The second inequality (b) is derived by using the upper bound of projection in   \eqref{eq:upper_bound_proj}, where $N$ is a dimension in the image space from volumetric data $S \times N \times N$. 
\end{proof}
Having the Lipschitz constant $L = 5 + 2\rho \sqrt{N}$, we can write the upper bound of the expected value given in the following lemma.
\begin{lemma}
\label{lemma: bound_prox_posterior}
The expected value of differences between $\mbf{x}_0$ and the proximal method, $\textcolor{black}{\mbf{\tilde x}_0 }= \text{prox}_{\alpha} \left( \mbf{\hat x}_0 - \lambda \nabla_{\mbf{\hat x}_0}\left(\widehat{L}\left(\mbf{\hat x}_0,  \rho \right)   \right) \right)$, with input posterior mean in Proposition \ref{prop:prop1}, $\mbf{\hat{x}}_0 := \E\left[\mbf{x}_0 | \mbf{x}_t\right]$ is upper bounded by  
$$
\E \left[\norm{\mbf{x}_0 - \mbf{\tilde x}_0}_2\right] \leq \left(\lambda \left(5 + 2\rho \sqrt{N} \right) + 1 \right)\E \left[\norm{\mbf{ x}_0 - \mbf{\hat x}_0 }_2\right], 
$$
where $N$ is the dimension of image space from volumetric data $S \times N \times N$, parameters $\lambda$ and $\rho$ are step size and multiplier, respectively. 
\end{lemma}
\begin{proof}
We start by writing the definition of proximal given posterior mean in Proposition \ref{prop:prop1} as follows
\begin{equation*} 
\begin{aligned}
\E \left[\norm{\mbf{x}_0 - \mbf{\tilde x}_0}\right] &=\E \left[\norm{\mbf{x}_0 -  {\text{prox}} \left(\mbf{\hat x}_0 - \lambda \nabla_{\mbf{\hat x}_0} \widehat{L}\left(\mbf{\hat x}_0,  \rho \right)  \right)}_2  \right] \\
&\stackrel{\text{(a)}}{=} \E \left[\norm{{\text{prox}} \left(\mbf{x}_0 - \lambda \nabla_{\mbf{x}_0} \widehat{L}\left(\mbf{x}_0,  \rho \right)  \right) -  {\text{prox}} \left(\mbf{\hat  x}_0 - \lambda \nabla_{\mbf{\hat x}_0} \widehat{L}\left(\mbf{\hat x}_0,  \rho \right)  \right)}_2  \right] \\
&\stackrel{\text{(b)}}{\leq}  \E \left[\norm{\mbf{x}_0 - \mbf{\hat x}_0 }_2\right] +  \lambda \E\left[\norm{\nabla_{\mbf{x}_0} \left(\widehat{L}\left(\mbf{x}_0,  \rho \right)  \right) - \nabla_{\mbf{\hat x}_0} \left(\widehat{L}\left(\mbf{\hat x}_0,  \rho \right)  \right)}_2 \right]\\
&\stackrel{\text{(c)}}{\leq}  \E \left[\norm{\mbf{ x}_0 - \mbf{\hat x}_0 }_2\right] +  \lambda (5 + 2\rho \sqrt{N})\E \left[\norm{\mbf{ x}_0 - \mbf{\hat x}_0 }_2\right]\\
&= \left(\lambda \left(5 + 2\rho \sqrt{N} \right) + 1 \right)\E \left[\norm{\mbf{ x}_0 - \mbf{\hat x}_0 }_2\right] 
\end{aligned}
\end{equation*}
\end{proof}
The equality (a) is derived from the definition of the proximal method in preserving the optimal solution, presented in Lemma \ref{lemma:prox_preserve}. The inequality (b) is given by the non-expansive property of proximal function in Lemma \ref{lemma:prox_non_expansive} and by adding the triangle inequality. The inequality (c) holds because of the Lipschitz constant $L = 5 + 2\rho \sqrt{N}$ in Lemma \ref{lemma:lipschitz_loss}.
To sum up, here we recall the main theorem presented in this paper to estimate $p(\mbf y| \mbf{x}_t) := \E\left[p(\mbf y|\mbf{x}_0)\right]$ as given in the main theorem, we restated here:
\begin{theorem} 
Suppose we have the update from proposed algorithm, namely $\textcolor{blue}{\mbf{\tilde x}_0 }= \text{prox}_{\alpha} \left( \mbf{\hat x}_0 - \lambda \nabla_{\mbf{\hat x}_0}\left(\widehat{L}\left(\mbf{\hat x}_0,  \rho \right)   \right) \right)$,  with $\mbf{\hat x}_0$ is the posterior mean given in Proposition \ref{prop:prop1} and step size $\lambda = \frac{1}{L}$ where $L$ is the Lipschitz constant of the loss function in Lemma \ref{lemma:lipschitz_loss}. Hence, we have
\begin{equation}
\card{ \E\left[p\left(\mbf{y} | \mbf{x}_0\right)\right]- p\left(\mbf{y} | \textcolor{blue}{\mbf{\tilde x}_0}\right)} \leq  \textcolor{blue}{\frac{e^{-\frac{1}{2}} }{\sqrt{\left(2\pi\right)^d\sigma^{2d + 2}}}} \underset{\mbf{x}}{\text{max}}\norm{\nabla_{\mbf{x}} \mcl{A}\left(\mbf{x}\right)}_2 \textcolor{blue}{m_2},
\end{equation}
where $\textcolor{blue}{m_2 = 2 m_1}$.
\end{theorem}
\begin{proof}
We start by writing the expected value in terms of multivariate Gaussian probability density function $\phi$
\begin{equation*}
\begin{aligned}
\card{ \E\left[p\left(\mbf{y} | \mbf{x}_0\right)\right]- p\left(\mbf{y} | \mbf{\tilde x}_0\right)} 
&\stackrel{\text{(a)}}{=}  \card{ \E\left[\phi\left(\mcl{A}\left(\mbf{x}_0 \right)\right) - \phi\left(\mcl{A}\left(\mbf{\tilde x}_0 \right)\right)\right]}\\
&\stackrel{\text{(b)}}{=}  \card{\int \phi\left(\mcl{A}\left(\mbf{x}_0 \right)\right) - \phi\left(\mcl{A}\left(\mbf{\tilde x}_0 \right)\right) p\left(\mbf{x}_0 | \mbf{x}_t \right) \mrm{d} \mbf{x}_0}\\
&\stackrel{\text{(c)}}{\leq}  \int \card{\phi\left(\mcl{A}\left(\mbf{x}_0 \right)\right) - \phi\left(\mcl{A}\left(\mbf{\tilde x}_0 \right)\right)} p\left(\mbf{x}_0 | \mbf{x}_t \right) \mrm{d} \mbf{x}_0\\
&\stackrel{\text{(d)}}{\leq} \frac{e^{-\frac{1}{2}} }{\sqrt{\left(2\pi\right)^d\sigma^{2d + 2}}}  \int \norm{\mcl{A}\left(\mbf{x}_0 \right)  - \mcl{A}\left(\mbf{\tilde x}_0 \right)}_2 p\left(\mbf{x}_0 | \mbf{x}_t \right) \mrm{d} \mbf{x}_0\\
&\stackrel{\text{(e)}}{\leq} \frac{e^{-\frac{1}{2}} }{\sqrt{\left(2\pi\right)^d\sigma^{2d + 2}}} \underset{\mbf{x}}{\text{max}}\norm{\nabla_{\mbf{x}} \mcl{A}\left(\mbf{x}\right)}_2 \E\left[\norm{ \mbf{x}_0  -  \mbf{\tilde x}_0 }_2\right]\\
&\stackrel{\text{(f)}}{\leq} \frac{e^{-\frac{1}{2}} }{\sqrt{\left(2\pi\right)^d\sigma^{2d + 2}}} \underset{\mbf{x}}{\text{max}}\norm{\nabla_{\mbf{x}} \mcl{A}\left(\mbf{x}\right)}_2 2\E \left[\norm{\mbf{ x}_0 - \mbf{\hat x}_0 }_2\right], 
\end{aligned}
\end{equation*}
where the first equality (a) is derived directly from the definition that both conditional probability density functions (pdf) $p\left(\mbf{y} | \mbf{x}_0\right), p\left(\mbf{y} | \mbf{\tilde x}_0\right)$ are Gaussian by incorporating the noisy forward model $\mbf{y} = \mcl{A}\left(\mbf{x} \right) + \mbf{n}$. The second equality (b) follows from the definition of expected value. Hence, we have upper bound by writing the inequality in (c) following the property of triangle inequality. The inequality in (d) is derived from the Lipschitz constant of the multivariate Gaussian pdf as discussed in Lemma \ref{lemma:multivar_gauss}. The inequality (e) follows from the mean value theorem where we can upper bound the forward function $\mcl A$ by having the maximum norm of the derivative with respect to the input of the forward function. The last inequality (f) is given from Lemma \ref{lemma:lipschitz_loss}, where we have Lipschitz constant $L = 5 + 2\rho \sqrt{N}$. To have the relation between the result from Diffusion Proximal Projection Method $\mbf{\tilde x}_0$ and posterior from DDPM sampling $\mbf{\hat x}_0$ the parameter $\lambda = \frac{1}{5 + 2\rho \sqrt{N} }$ is chosen.
$$
\E \left[\norm{\mbf{ x}_0 - \mbf{\tilde  x}_0 }_2\right] \leq 2 \E \left[\norm{\mbf{ x}_0 - \mbf{\hat  x}_0 }_2\right] = 2m_1
$$
\end{proof}
\subsection{Additional Experimental Results}
In this section, we perform additional experimental results to compare all methods discussed in the main article. Here we present the reconstruction for all data, including fastMRI knee \cite{zbontar2018fastmri}, BRATS \cite{menze2014multimodal, bakas2017advancing, bakas2018identifying}, as well as the plant roots datasets.
\begin{figure*}[ht!]
    \centering
    \includesvg[width=0.95\textwidth]{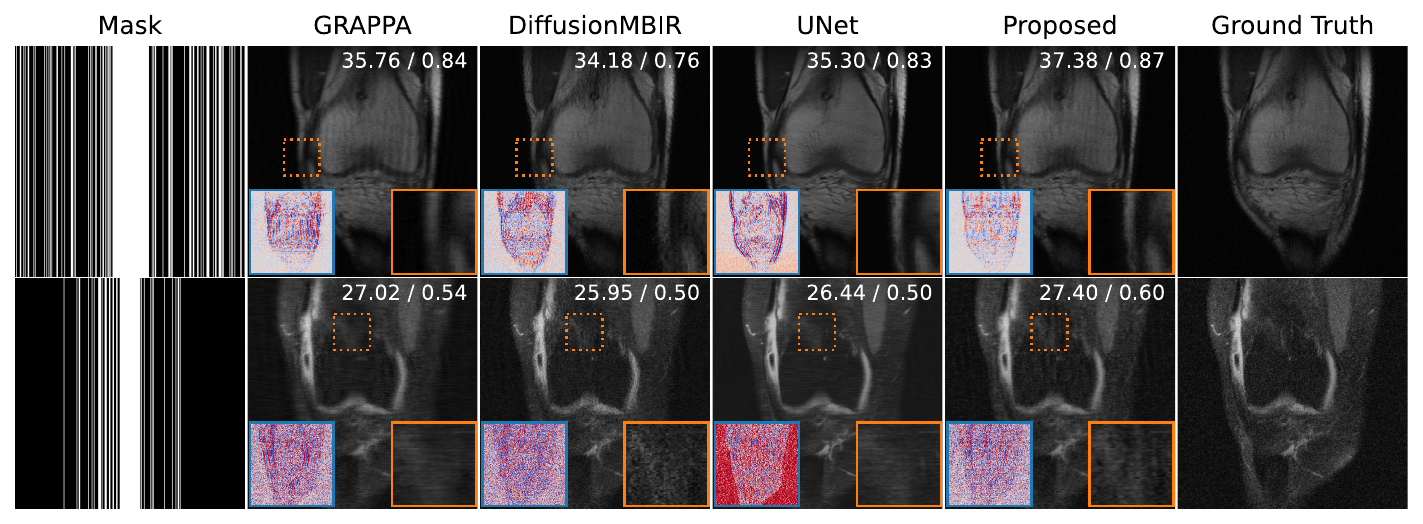}
     \caption{Single slice from the volume reconstruction of file1000660 (top) and file1000026 (bottom) from fastMRI knee data. 
    % (a) Mask or Under-sampling operator, (b) GRAPPA \cite{griswold2002generalized}, (c) DiffusionMBIR \cite{chung2023solving}, (d) U-Net \cite{unetmri2017}, (e) Proposed Method, (f) Ground Truth. 
    The numbers on the top right corner represent the PSNR/SSIM of the slice. The subplots on the lower left corner represent the difference map between the reconstruction and ground truth. The color range is between $-0.02$ (bluish) and $0.02$ (reddish). Note that the volumetric ground truth data has been normalized. The subplots on the lower right are a zoomed-in view.}
\label{Fig:knee_supp}
\end{figure*}
% \begin{figure*}[t!]
%     \centering
%     % \includegraphics[scale=0.8]{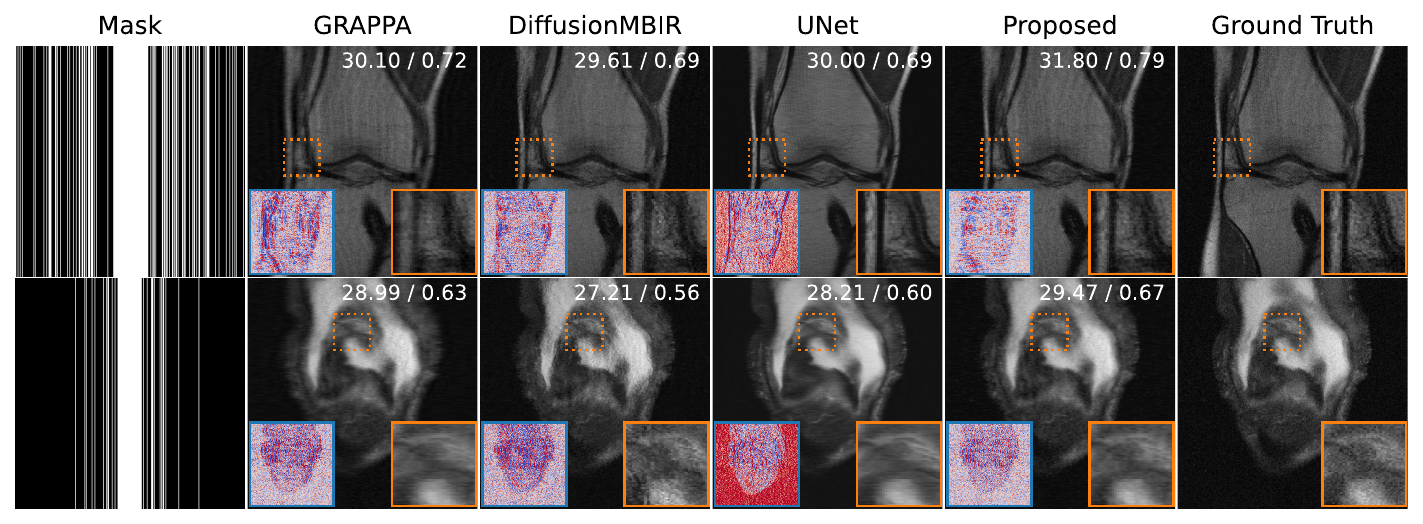}
%     \includesvg[width=0.95\textwidth]{Figure/compare_root_3D.svg}
%     \caption{Reconstructions for roots data form Lotus plant. (a) Mask or Under-sampling operator, (b) GRAPPA \cite{griswold2002generalized}, (c) Diffusion MBIR \cite{chung2023solving}, (d) U-Net \cite{unetmri2017}, (e) Proposed Method, (f) Ground Truth.}
% \label{Fig:lotus_3d}
% \end{figure*}
Similar performance can be observed for BRATS and plant roots data, where we have higher SSIM and PSNR, given in \Cref{Fig:brats_supp} and \Cref{Fig:root_supp}. Additionally, the error differences provided in the zoomed subplots in left bottom corner show that the proposed algorithm produce smaller background error compared to other algorithms. 
\Cref{Fig:knee_supp} shows the slice reconstruction of another knee dataset for all methods compared in this paper. It can be seen that the proposed method outperforms other methods in terms of SSIM and PSNR for both Uniform and Gaussian masking.
\begin{figure*}[t]
    \centering
    \includesvg[width=0.8\textwidth]{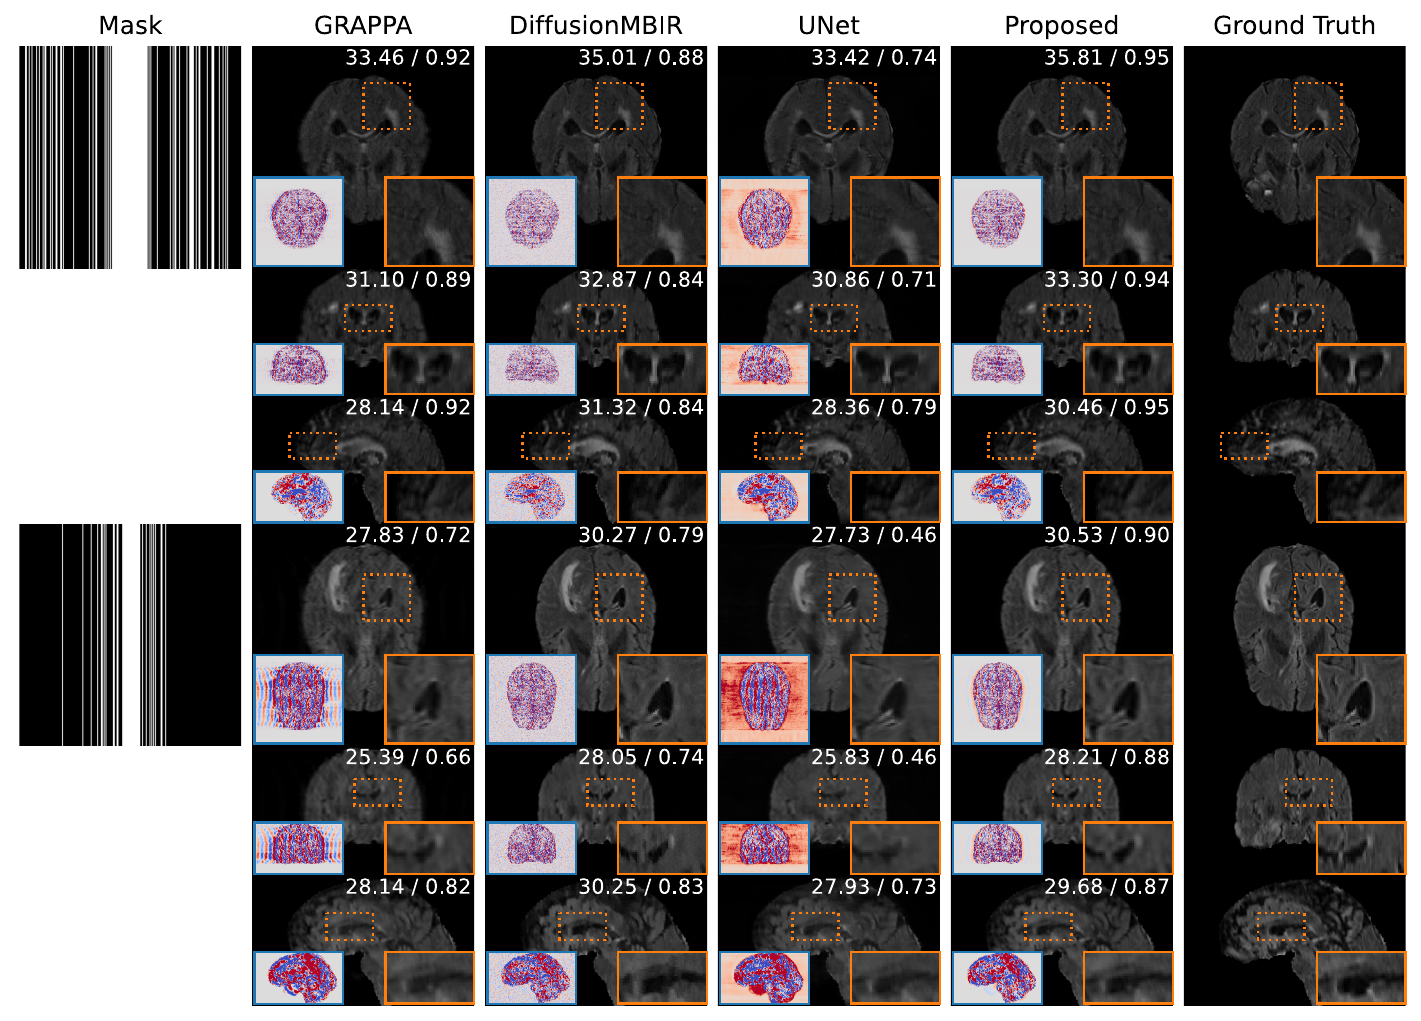}
      \caption{Slices from the volume reconstructions for BRATS data from Brats18\_CBICA\_AUC\_1 (top) and Brats18\_CBICA\_AAM\_1 (bottom). 
    We present vertically the axial, sagittal, and coronal middle slices. The numbers on the upper right of each image represent the PSNR/SSIM of the middle slices. The subplots on the lower left are the difference map of the projection w.r.t. the ground truth. The color range is between $-0.02$  (bluish) and $0.02$ (reddish).}
\label{Fig:brats_supp}
\end{figure*}
\begin{figure*}[b]
    \centering
    \includesvg[width=0.8\textwidth]{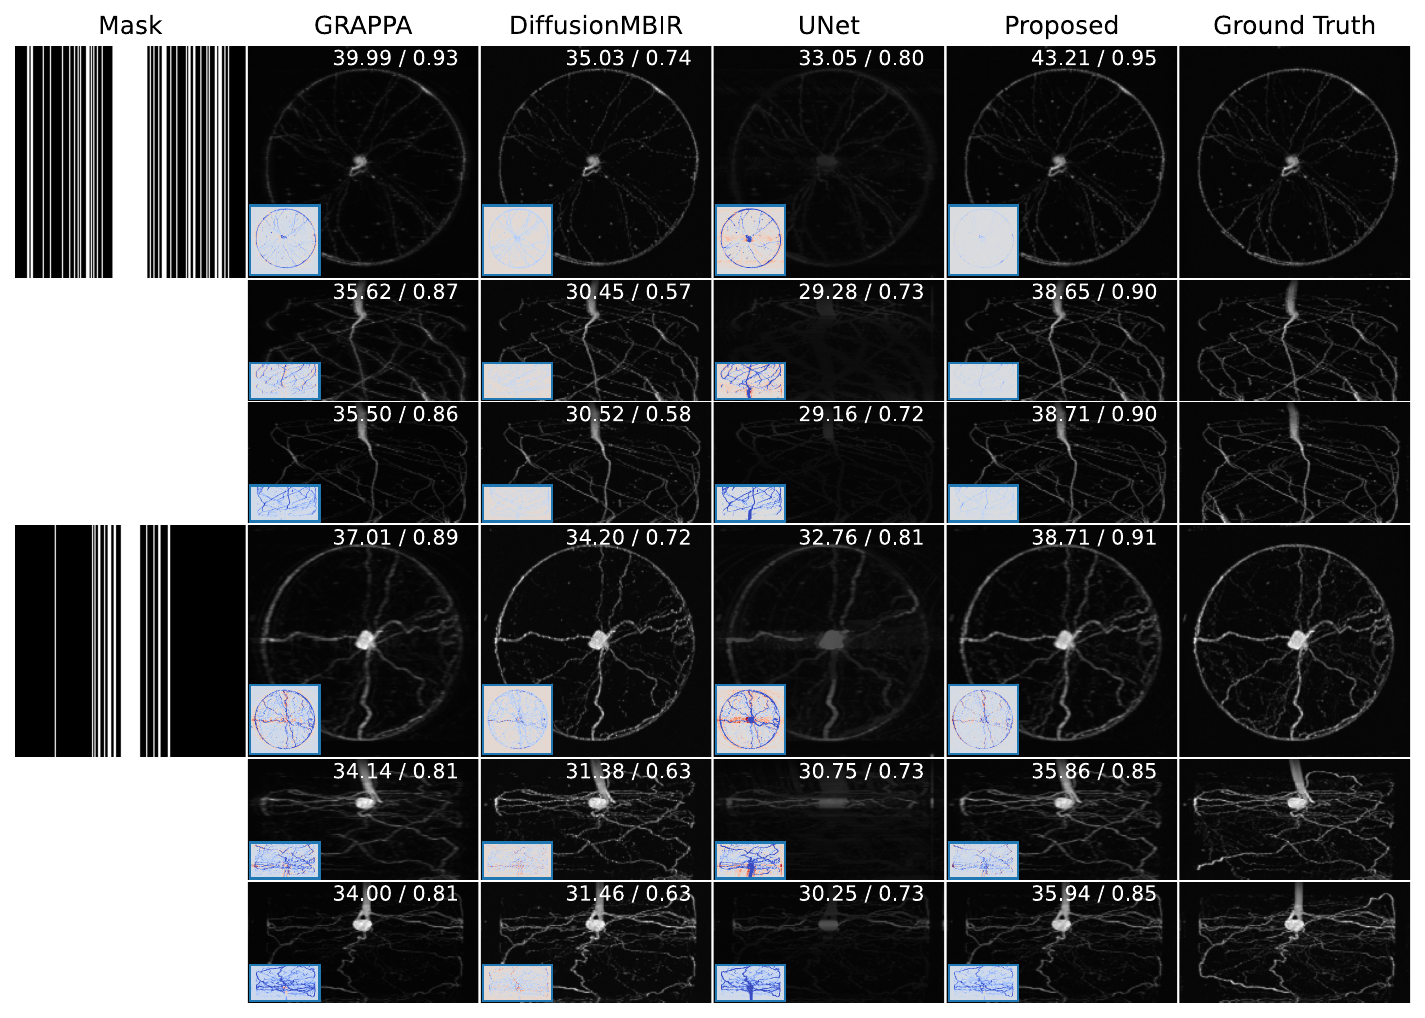}
     \caption{Reconstructions for Soja (top) and Maize (bottom) plant roots data.
    We present vertically the axial, coronal, and sagittal maximum intensity projections. The numbers on the upper right of each image represent the mean PSNR/SSIM of slices along dimensions. The subplots on the lower left are the difference map of the projection w.r.t. the ground truth. The color range is between $-0.1$ (bluish) and $0.1$ (reddish).}
\label{Fig:root_supp}
\end{figure*}
In \Cref{tab:testset}, we provide the list of data we used to generate the evaluation results in \Cref{tab:result_knee} and \ref{tab:result_roots}.
\begin{table}[tb]
\centering
\caption{The test sets used for evaluation experiments corresponding to \Cref{tab:result_knee} and \Cref{tab:result_roots}.}
\label{tab:testset}
\resizebox{0.8\textwidth}{!}{%
\begin{tabular}{l @{\hskip 0.3in} l @{\hskip 0.3in}l}
\toprule
\multicolumn{3}{c}{Test set}                               \\ \cmidrule[0.5pt](rl){1-3}
Knee           & BRATS                      & Root           \\ \hline
file1000026 & Brats18\_CBICA\_AAM\_1  & barley1      \\
file1000114 & Brats18\_CBICA\_ABT\_1  & barley25     \\
file1000178 & Brats18\_CBICA\_ALV\_1  & lotus        \\
file1000308 & Brats18\_CBICA\_APM\_1  & maize1       \\
file1000323 & Brats18\_CBICA\_ATW\_1  & maize18      \\
file1000528 & Brats18\_CBICA\_AUC\_1  & maize26      \\
file1000660 & Brats18\_CBICA\_AUE\_1  & maize28      \\
file1000748 & Brats18\_CBICA\_BHN\_1  & mix\_data108 \\
file1000758 & Brats18\_MDA\_1012\_1   & mix\_data128 \\
file1000817 & Brats18\_MDA\_1081\_1   & mix\_data137 \\
file1000891 & Brats18\_MDA\_922\_1    & mix\_data177 \\
file1001096 & Brats18\_TCIA03\_604\_1 & mix\_data209 \\
file1001104 & Brats18\_TCIA07\_601\_1 & mix\_data217 \\
file1001140 & Brats18\_TCIA07\_602\_1 & mix\_data268 \\
file1001163 & Brats18\_TCIA09\_248\_1 & mix\_data275 \\
file1001184 & Brats18\_TCIA11\_612\_1 & mix\_data297 \\
file1001219 & Brats18\_TCIA12\_613\_1 & mix\_data307 \\
file1001289 & Brats18\_TCIA13\_611\_1 & mix\_data42  \\
file1001298 & Brats18\_TCIA13\_617\_1 & mix\_data423 \\
file1001365 & Brats18\_TCIA13\_636\_1 & mix\_data58  \\
file1001598 & Brats18\_TCIA13\_638\_1 & mix\_data70  \\
file1001825 & Brats18\_TCIA13\_646\_1 & mix\_data82  \\
file1001834 & Brats18\_UAB\_3449\_1   & soja29       \\
file1001862 & Brats18\_UAB\_3454\_1   & soja66       \\
file1001938 & Brats18\_UAB\_3456\_1   & vicia        \\
file1001977 & Brats18\_UAB\_3490\_1   &              \\
file1002155 & Brats18\_WashU\_S037\_1 &              \\
file1002257 & Brats18\_WashU\_S041\_1 &              \\
file1002340 & Brats18\_WashU\_W033\_1 &              \\
file1002436 & Brats18\_WashU\_W038\_1 &              \\ \bottomrule
\end{tabular}%
}
\end{table}
